# Supplementary material for: Behavior Priors for Efficient Reinforcement Learning
Source: arXiv:2010.14274 source file (2020-10-27)
Supplement: Supplementary file 1 [file appendix_general.tex]

\section{A general framework for RL as probabilistic modelling}
\dhruva{DOUBLE Check: Can we include Leonards results?}
\label{appendix:general_framework}

In Sections~\ref{sec:prob_rl} and~\ref{sec:hierarchy:KL} of the main text we have introduced the KL-regularized objective and explored a particular formulation that uses latent variables in the default policy and policy (Section~\ref{sec:hierarchy:KL} and experiments). The particular choice in Section~\ref{sec:hierarchy:KL} arises as a special case of a more general framework which we here outline briefly. 

For both the default policy and for agent policy we can consider general directed latent variable models of the following form
\begin{align}
\pp(\tau) &= \textstyle \int \pp(\tau| y) \pp(y) d y,\\
\qq(\tau) &= \textstyle \int \qq(\tau | z) \qq(z) d z
\end{align}
where both $y$ and $z$ can be time varying, e.g.\ $y=(y_1, \dots y_T)$, and can be causally dependent on the trajectory prefix $x_t$, e.g.\ $y_t \sim p(\cdot | x_t)$ (and equivalently for $z$). The latent variables can further be continuous or discrete, and $y_t$ or $z_t$ can exhibit further structure (and thus include e.g.~binary variables that model option termination). %Different model structures will give rise to models with different biases. \nicolas{example here?}
The general form of the objective presented in the main text
\begin{align}
\textstyle
\mathcal{L}(\qq, \pp) & = \textstyle \EE_{\tau} \left[ 
\sum_{t\ge1}  \gamma^t r(s_t,a_t) 
      - \alpha \gamma^t \KL(a_t|x_t) \right],
\nonumber %\label{eq:objective:KL_regularized:appendix}
\end{align}
 remains valid regardless of the particular form of $\pp$ and $\qq$.
This form can be convenient when $\pp(a_t | x_t)$ and $\qq(a_t | x_t)$ are tractable (e.g.\ when $z$ or $y$ have a small number of discrete states or decompose conveniently over time, e.g.~as in \cite{fox2017multi,krishnan2017discovery}).

%Similar to the situation in the probabilistic modeling literature where a given model can often be optimized with a number of different algorithms and approximations, a particular instance of the the regularized objective (\ref{eq:objective:KL_regularized}) will admit different algorithmic solutions which, in general, will alternate between optimizing $\qq$ as a regularized RL problem, and $\pp$ as a density estimation problem, akin to the E- and M-steps in the expectation-maximization algorithm \cite{dempsterXXX}. 

In general, however, latent variables in $\pp$ and $\qq$ may 
%render $\pp(a_t | x_t)$ and $\qq(a_t | x_t)$ intractable and 
introduce the need for additional approximations. In this case different models and algorithms can be instantiated based on a) the particular approximation chosen there, as well as b) choices for sharing of components between $\pp$ and $\qq$.
A possible starting point when $\pp$ contains latent variables is the following lower bound to $\mathcal{L}$:
\begin{align}
\mathcal{L} 
&= \textstyle \EE_\qq[ \sum_t r(s_t,a_t)] - 
\KL[ \qq(\tau) || \pp(\tau) ]\\
%&\geq \textstyle \EE_\qq \left [ \sum_t r(s_t,a_t) + \EE_f \left [ \log \pp(\tau) + \frac{\pp(y)}{f(y|\tau)} \right ] \right] + \Ent [ \qq(\tau) ]\\
%&{\color{blue}\geq \textstyle \EE_\qq \left [ \sum_t r(s_t,a_t) + \EE_f \left [ \log \pp(\tau) + \frac{\pp(y)}{f(y|\tau)} \right ] \right] + \Ent [ \qq(\tau) ] (??)}\\
&\geq \textstyle \EE_\qq \left [ \sum_t r(s_t,a_t) + \EE_f \left [ \log\frac{\pp(\tau,y)}{f(y|\tau)} \right ] \right] + \Ent [ \qq(\tau) ]\\
&= \textstyle \EE_\qq\left [ \sum_t r(s_t,a_t) + \EE_f \left [ \log \pp(\tau|y) \right ] \right. \nonumber\\
&\hspace{1.8cm}-\left. \KL [ f(y|\tau) || \pp(y) ] \right] + \Ent [ \qq(\tau) ]. \label{eq:objective:prior_ELBO}
\end{align}
If $y_t$ are discrete and take on a small number of values we can compute $f(y|\tau)$ exactly (e.g.~using the forward-backward algorithm as in \cite{fox2017multi,krishnan2017discovery}); in other cases we can learn a parameterized approximation to the true posterior or can conceivably apply mixed inference schemes \citep[e.g.][]{johnson2016composing}.

Latent variables in the policy $\qq$ can require an alternative approximation discussed e.g.\ in \cite{hausman2018learning}:
\begin{equation}
\begin{split}
    \mathcal{L} 
\geq \textstyle \EE_\qq\big[ &\textstyle\sum_t r(s_t,a_t) +  \log \pp(\tau) + \log g(z | \tau)  \\
&\textstyle+  \Ent [ \qq(\tau| z) ]   \big] + \Ent [ q(Z)], 
\label{eq:objective:KL_prior_posterior}
\end{split}
\end{equation}
where $g$ is a learned approximation to the true posterior $\qq(z|\tau)$. 
(But see e.g.\ \cite{haarnoja2018latent} who consider a parametric form for policies with latent variables for which the entropy term can be computed analytically and no approximation is needed.)
This formulation bears interesting similarities with diversity inducing regularization schemes based on mutual information \citep[e.g.][]{gregor2016variational,florensa2017stochastic} but arises here as an approximation to trajectory entropy. This formulation also has interesting connections to auxiliary variable formulations in the approximate inference literature \cite{salimans2014bridging,agakov2004an}.  %Note that although $g$ approximates a posterior similar to $f$ its role is rather different and it can be seen as a learned intrinsic reward that encourages the overall identifiability of $z$ from the resulting trajectory. 

When both $\pp$ and $\qq$ contain latent variables eqs. (\ref{eq:objective:prior_ELBO},\ref{eq:objective:KL_prior_posterior}) can be combined. The model described in Section~\ref{sec:hierarchy:KL} in the main text then arises when the latent variable is ``shared'' between $\pp$ and $\qq$ and we effectively use the policy itself as the inference network for $\pp$: $f(y| \tau) = \prod_t \qq(y_t | x_t)$. In this case the objective simplifies to
\begin{align}
\textstyle \mathcal{L} 
&\geq \textstyle \EE_\qq\left [ \sum_t r(s_t,a_t) +  \log \frac{\pp(\tau|z)\pp(z)}{\qq(\tau|z)\qq(z)} \right ].
\end{align}
When we further set $\pp(\tau|z) = \qq(\tau|z)$ we recover the model discussed in the main text of the paper.

As a proof-of-concept for a model without a shared latent space, with latent variables in $\pi_0$ but not $\pi$, we consider a simple humanoid with 28 degrees of freedom and 21 actuators and consider two different tasks: 1) a dense-reward walking task, in which the agent has to move forward, backward, left, or right at a fixed speed. The direction is randomly sampled at the beginning of an episode and changed to a different direction half-way through the episode and 2) a sparse reward go-to-target task, in which the agent has to move to a target whose location is supplied to the agent as a feature vector similar to those considered in \cite{galashov2018information}.

\begin{figure*}
    \centering
    \includegraphics[width=0.95\linewidth]{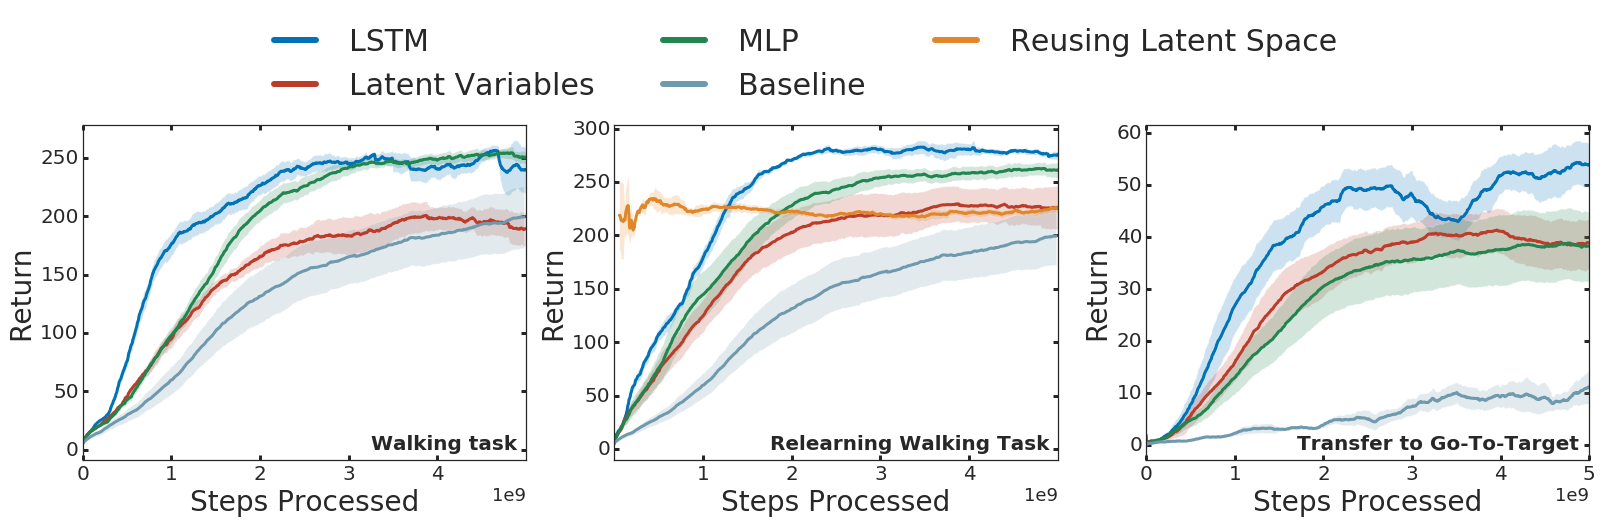}
    \caption{
        \textbf{Results with a latent variable prior.} \textbf{Left}: Walking task with the simple humanoid \textbf{Center}: Relearning the walking task with fixed priors. \textbf{Right}: Transfer to a go-to-target task.
    }
    \label{fig:latent_variables_in_prior}
\end{figure*}

Figure \ref{fig:latent_variables_in_prior} shows some exploratory results. In a first experiment we compare different prior architectures on the directional walking task. We let the prior marginalize over task condition. We include a feed-forward network, an LSTM, and a latent variable model with one latent variable per time step in the comparison. For the latent variable model we chose an inference network $f(z_t|z_{t-1}, \tau)$ so that eq.\ \eqref{eq:objective:prior_ELBO} decomposes over time. All priors studied in this comparison gave a modest speed-up in learning. While the latent variable prior works well, it does not work as well as the LSTM and MLP priors in this setup.
In a first set of transfer experiments, we used the learned priors to learn the walking task again. Again, the learned priors led to a modest speed-up relative to learning from scratch. 

We also experimented with parameter sharing for transfer as in the main text. We can freeze the conditional distribution $\pp(a|s, z)$ and learn a new policy $\qq(z|s)$, effectively using the learned latent space as an action space. 
In a second set of experiments, we study how well a prior learned on the walking task can transfer to the sparse go-to-target task. Here all learned priors led to a significant speed up relative to learning from scratch. Small return differences aside, all three different priors considered here solved the task with clear goal directed movements. On the other hand, the baseline only learned to go to very close-by targets. Reusing the latent space did not work well on this task. We speculate that the required turns are not easy to represent in the latent space resulting from the walking task.
