# Supplementary material for: Behavior Priors for Efficient Reinforcement Learning
Source: arXiv:2010.14274 source file (2020-10-27)
Supplement: Supplementary file 2 [file algorithm.tex]

\section{Algorithms}
\label{appendix:algorithm}
